# Supplementary material for: Efficient Few-Shot Fine-Tuning for Opinion Summarization
Source: arXiv:2205.02170 source file (2022-05-08)
Supplement: Supplementary file 1 [file error_analysis.tex]

\subsection{Error Analysis}
\label{app:error_analysis}
