# Supplementary material for: Efficient Few-Shot Fine-Tuning for Opinion Summarization
Source: arXiv:2205.02170 source file (2022-05-08)
Supplement: Supplementary file 2 [file pov_analysis.tex]

\subsection{POV Analysis}
\label{app:pov_analysis}

Here is the POV analysis.

\begin{table*}[h!]
    \centering
    \small
    \begin{tabular}{ l | c c c c | c c c c}
    \multicolumn{1}{c}{} & \multicolumn{4}{c}{\textbf{Amazon}} & \multicolumn{4}{c}{\textbf{Yelp}} \\ \thickhline
     & 1st & 2nd & 3rd & NoPr & 1st & 2nd & 3rd & NoPr \\
    \thickhline
        \textsc{Gold} & 0.00 & 1.67 & 60.00 & 38.33 & - & - & - & - \\
        \thickhline
    \textsc{MeanSum}~\citep{chu2019meansum} & - & - & - & - & - & - & - & - \\
    \textsc{Copycat}~\citep{brazinskas2020-unsupervised} & 48.42 & 0.00 & 51.58 & 0.00 & - & - & - & - \\ 
    \thickhline 
    \multicolumn{9}{c}{\textit{Few-shot}} \\ \thickhline 
    \textsc{FewSum}~\citep{brazinskas2020few} & 0.50 & 1.33 & 83.17 & 15.00 & - & - & - & - \\
    \textsc{PASS}~\citep{Oved2021PASSPS} & 0.00 & 0.00 & 75.00 & 25.00 & - & - & - & - \\ 
    % \thickhline 
    % \multicolumn{9}{c}{\textit{Ours}} \\ \thickhline 
    \textsc{Full (100\%)} & 1.67 & 8.33 & 45.00 & 45.00 & - & - & - & - \\
    \textsc{Full (100\%) + l1o} & 5.00 & 3.33 & 26.67 & 65.00 & - & - & - & - \\
    \adasum{5} & 5.00 & 7.50 & 47.50 & 40.00 & - & - & - & - \\
    \adasumloo{5} & 0.00 & 14.72 & 45.28 & 40.00 & - & - & - & - \\
    \adasumloo{5}$^{*}$ & 1.00 & 8.92 & 55.08 & 35.00 & - & - & - & - \\
    \thickhline
    \end{tabular}
    \caption{.}
    \label{table:pov_analysis}
\end{table*}
